# Supplementary material for: CASIA-Face-Africa: A Large-scale African Face Image Database
Source: arXiv:2105.03632 source file (2021-05-11)
Supplement: Supplementary file 1 [file appendix.pdf]

TABLE I

1:1 VERIFICATION RESULTS AT VARIOUS VALUES OF FAR OF ID-V-SPLIT- PROTOCOLS WITH AND WITHOUT ALIGNMENT

| Algorithm | ID-V-Split-Ep1 | | | | ID-V-Split-Ep2 | | | | ID-V-Split-Ep3 | | | |
|---|---|---|---|---|---|---|---|---|---|---|---|---|
| | FAR=0.1% | | FAR=1% | | FAR=0.1% | | FAR=1% | | FAR=0.1% | | FAR=1% | |
| | Without | With | Without | With | Without | With | Without | With | Without | With | Without | With |
| ArcFace(r34-amf) | $15.0 \pm 1.5$ | $13.3 \pm 1.1$ | $25.7 \pm 2.4$ | $24.5 \pm 1.7$ | $0.0 \pm 0.0$ | $0.0 \pm 0.0$ | $0.3 \pm 0.1$ | $0.0 \pm 0.0$ | $0.0 \pm 0.0$ | $0.0 \pm 0.0$ | $1.0 \pm 0.7$ | $0.6 \pm 0.3$ |
| ArcFace(r50-am-lfw) | $16.3 \pm 1.8$ | $10.8 \pm 1.1$ | $27.0 \pm 1.6$ | $22.1 \pm 2.4$ | $0.1 \pm 0.2$ | $0.0 \pm 0.0$ | $0.7 \pm 0.3$ | $0.1 \pm 0.1$ | $0.2 \pm 0.2$ | $0.0 \pm 0.0$ | $1.9 \pm 1.2$ | $0.6 \pm 0.2$ |
| ArcFace(r100-ii) | $19.4 \pm 1.5$ | $13.6 \pm 1.7$ | $31.9 \pm 2.0$ | $25.7 \pm 1.5$ | $0.3 \pm 0.3$ | $0.1 \pm 0.1$ | $2.3 \pm 0.9$ | $1.0 \pm 0.3$ | $0.5 \pm 0.3$ | $0.3 \pm 0.1$ | $3.5 \pm 0.9$ | $2.3 \pm 0.6$ |
| SphereFace | $16.6 \pm 1.5$ | $19.8 \pm 1.6$ | $27.8 \pm 2.7$ | $30.1 \pm 2.1$ | $0.0 \pm 0.0$ | $0.0 \pm 0.0$ | $0.0 \pm 0.0$ | $0.0 \pm 0.0$ | $0.0 \pm 0.0$ | $0.0 \pm 0.0$ | $0.0 \pm 0.0$ | $0.0 \pm 0.0$ |
| lightCNN-29-V2 | $74.2 \pm 2.3$ | $63.5 \pm 3.0$ | $83.5 \pm 2.0$ | $76.2 \pm 2.1$ | $10.9 \pm 0.7$ | $6.2 \pm 1.0$ | $32.6 \pm 3.2$ | $20.7 \pm 2.3$ | $13.0 \pm 1.3$ | $9.3 \pm 1.3$ | $34.0 \pm 4.0$ | $27.7 \pm 2.0$ |
| lightCNN-29 | $63.8 \pm 1.3$ | $49.4 \pm 3.0$ | $75.1 \pm 2.4$ | $63.6 \pm 1.9$ | $3.8 \pm 0.7$ | $1.1 \pm 0.4$ | $15.0 \pm 1.0$ | $5.4 \pm 0.6$ | $6.1 \pm 0.7$ | $1.5 \pm 0.6$ | $18.6 \pm 1.1$ | $8.5 \pm 1.2$ |
| lightCNN-9 | $37.1 \pm 1.9$ | $35.9 \pm 2.6$ | $52.1 \pm 1.8$ | $48.7 \pm 2.1$ | $0.1 \pm 0.2$ | $0.0 \pm 0.0$ | $0.8 \pm 0.3$ | $0.1 \pm 0.1$ | $0.3 \pm 0.1$ | $0.1 \pm 0.1$ | $3.1 \pm 0.7$ | $1.6 \pm 0.6$ |
| Balanced-Softmax | $15.8 \pm 1.1$ | $19.3 \pm 1.4$ | $28.1 \pm 1.7$ | $32.4 \pm 1.7$ | $0.0 \pm 0.0$ | $0.0 \pm 0.0$ | $0.6 \pm 0.4$ | $0.1 \pm 0.2$ | $0.1 \pm 0.2$ | $0.1 \pm 0.1$ | $1.4 \pm 0.2$ | $0.6 \pm 0.3$ |
| CASIA-Arcface | $0.8 \pm 0.3$ | $1.1 \pm 0.2$ | $3.4 \pm 0.2$ | $5.2 \pm 0.3$ | $0.0 \pm 0.0$ | $0.0 \pm 0.0$ | $0.0 \pm 0.0$ | $0.0 \pm 0.0$ | $0.0 \pm 0.0$ | $0.0 \pm 0.0$ | $0.0 \pm 0.0$ | $0.0 \pm 0.0$ |
| CASIA-Softmax | $8.2 \pm 0.8$ | $5.6 \pm 0.8$ | $17.7 \pm 0.7$ | $14.7 \pm 1.5$ | $0.0 \pm 0.0$ | $0.0 \pm 0.0$ | $0.1 \pm 0.1$ | $0.0 \pm 0.0$ | $0.0 \pm 0.0$ | $0.0 \pm 0.0$ | $0.0 \pm 0.0$ | $0.0 \pm 0.0$ |
| Global-Softmax | $9.5 \pm 1.0$ | $6.9 \pm 1.6$ | $20.5 \pm 1.7$ | $20.3 \pm 2.2$ | $0.1 \pm 0.1$ | $0.0 \pm 0.0$ | $1.0 \pm 0.3$ | $0.1 \pm 0.1$ | $0.0 \pm 0.0$ | $0.1 \pm 0.1$ | $0.8 \pm 0.1$ | $0.5 \pm 0.3$ |
| MS1M-Arcface | $9.1 \pm 1.1$ | $6.3 \pm 0.8$ | $17.8 \pm 1.0$ | $15.3 \pm 1.7$ | $0.0 \pm 0.0$ | $0.0 \pm 0.0$ | $0.1 \pm 0.1$ | $0.2 \pm 0.3$ | $0.0 \pm 0.0$ | $0.1 \pm 0.1$ | $0.4 \pm 0.2$ | $0.5 \pm 0.4$ |

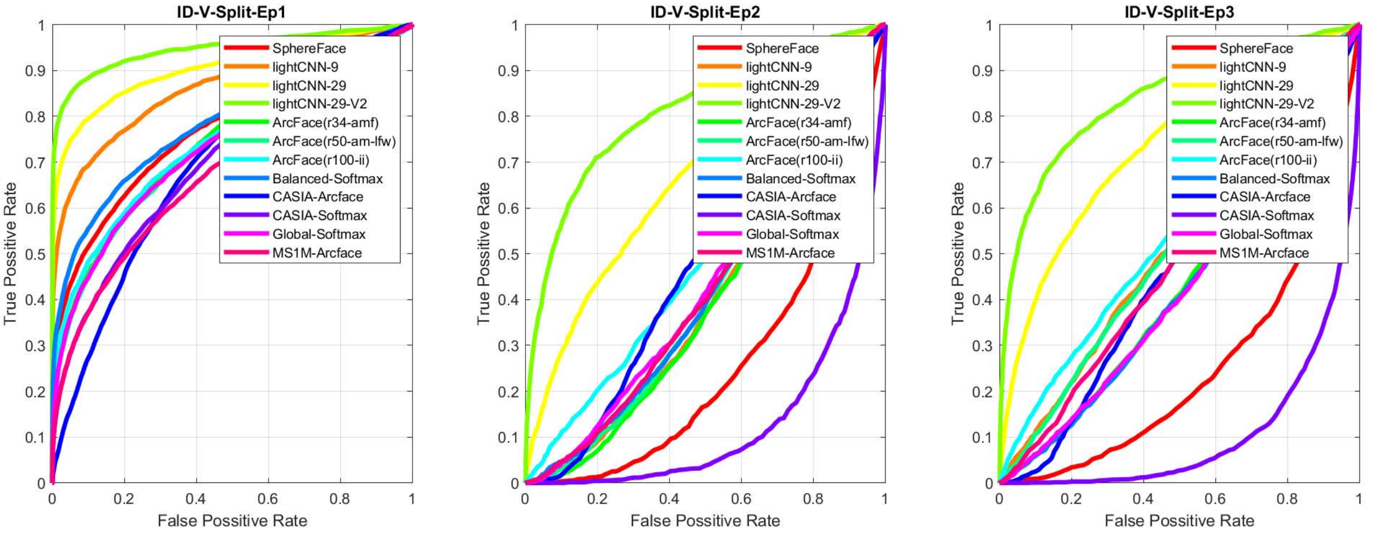


(a) (b) (c)

Fig. 1. Verification ROC curves for the protocols: (a) ID-V-Split-Ep1, (b) ID-V-Split-Ep2, (c) ID-V-Split-Ep3

,

TABLE II

1:1 VERIFICATION RESULTS AT VARIOUS VALUES OF FAR OF ID-V-SPLIT- PROTOCOLS WITH AND WITHOUT ALIGNMENT

| Algorithm | ID-V-Split-Ep1 | | | | ID-V-Split-Ep2 | | | | ID-V-Split-Ep3 | | | |
|---|---|---|---|---|---|---|---|---|---|---|---|---|
| | FAR=0.1% | | FAR=1% | | FAR=0.1% | | FAR=1% | | FAR=0.1% | | FAR=1% | |
| | Without | With | Without | With | Without | With | Without | With | Without | With | Without | With |
| ArcFace(r34-amf) | $15.0 \pm 1.5$ | $13.3 \pm 1.1$ | $25.7 \pm 2.4$ | $24.5 \pm 1.7$ | $0.0 \pm 0.0$ | $0.0 \pm 0.0$ | $0.3 \pm 0.1$ | $0.0 \pm 0.0$ | $0.0 \pm 0.0$ | $0.0 \pm 0.0$ | $1.0 \pm 0.7$ | $0.6 \pm 0.3$ |
| ArcFace(r50-am-lfw) | $16.3 \pm 1.8$ | $10.8 \pm 1.1$ | $27.0 \pm 1.6$ | $22.1 \pm 2.4$ | $0.1 \pm 0.2$ | $0.0 \pm 0.0$ | $0.7 \pm 0.3$ | $0.1 \pm 0.1$ | $0.2 \pm 0.2$ | $0.0 \pm 0.0$ | $1.9 \pm 1.2$ | $0.6 \pm 0.2$ |
| ArcFace(r100-ii) | $19.4 \pm 1.5$ | $13.6 \pm 1.7$ | $31.9 \pm 2.0$ | $25.7 \pm 1.5$ | $0.3 \pm 0.3$ | $0.1 \pm 0.1$ | $2.3 \pm 0.9$ | $1.0 \pm 0.3$ | $0.5 \pm 0.3$ | $0.3 \pm 0.1$ | $3.5 \pm 0.9$ | $2.3 \pm 0.6$ |
| SphereFace | $16.6 \pm 1.5$ | $19.8 \pm 1.6$ | $27.8 \pm 2.7$ | $30.1 \pm 2.1$ | $0.0 \pm 0.0$ | $0.0 \pm 0.0$ | $0.0 \pm 0.0$ | $0.0 \pm 0.0$ | $0.0 \pm 0.0$ | $0.0 \pm 0.0$ | $0.0 \pm 0.0$ | $0.0 \pm 0.0$ |
| lightCNN-29-V2 | $74.2 \pm 2.3$ | $63.5 \pm 3.0$ | $83.5 \pm 2.0$ | $76.2 \pm 2.1$ | $10.9 \pm 0.7$ | $6.2 \pm 1.0$ | $32.6 \pm 3.2$ | $20.7 \pm 2.3$ | $13.0 \pm 1.3$ | $9.3 \pm 1.3$ | $34.0 \pm 4.0$ | $27.7 \pm 2.0$ |
| lightCNN-29 | $63.8 \pm 1.3$ | $49.4 \pm 3.0$ | $75.1 \pm 2.4$ | $63.6 \pm 1.9$ | $3.8 \pm 0.7$ | $1.1 \pm 0.4$ | $15.0 \pm 1.0$ | $5.4 \pm 0.6$ | $6.1 \pm 0.7$ | $1.5 \pm 0.6$ | $18.6 \pm 1.1$ | $8.5 \pm 1.2$ |
| lightCNN-9 | $37.1 \pm 1.9$ | $35.9 \pm 2.6$ | $52.1 \pm 1.8$ | $48.7 \pm 2.1$ | $0.1 \pm 0.2$ | $0.0 \pm 0.0$ | $0.8 \pm 0.3$ | $0.1 \pm 0.1$ | $0.3 \pm 0.1$ | $0.1 \pm 0.1$ | $3.1 \pm 0.7$ | $1.6 \pm 0.6$ |
| Balanced-Softmax | $15.8 \pm 1.1$ | $19.3 \pm 1.4$ | $28.1 \pm 1.7$ | $32.4 \pm 1.7$ | $0.0 \pm 0.0$ | $0.0 \pm 0.0$ | $0.6 \pm 0.4$ | $0.1 \pm 0.2$ | $0.1 \pm 0.2$ | $0.1 \pm 0.1$ | $1.4 \pm 0.2$ | $0.6 \pm 0.3$ |
| CASIA-Arcface | $0.8 \pm 0.3$ | $1.1 \pm 0.2$ | $3.4 \pm 0.2$ | $5.2 \pm 0.3$ | $0.0 \pm 0.0$ | $0.0 \pm 0.0$ | $0.0 \pm 0.0$ | $0.0 \pm 0.0$ | $0.0 \pm 0.0$ | $0.0 \pm 0.0$ | $0.0 \pm 0.0$ | $0.0 \pm 0.0$ |
| CASIA-Softmax | $8.2 \pm 0.8$ | $5.6 \pm 0.8$ | $17.7 \pm 0.7$ | $14.7 \pm 1.5$ | $0.0 \pm 0.0$ | $0.0 \pm 0.0$ | $0.1 \pm 0.1$ | $0.0 \pm 0.0$ | $0.0 \pm 0.0$ | $0.0 \pm 0.0$ | $0.0 \pm 0.0$ | $0.0 \pm 0.0$ |
| Global-Softmax | $9.5 \pm 1.0$ | $6.9 \pm 1.6$ | $20.5 \pm 1.7$ | $20.3 \pm 2.2$ | $0.1 \pm 0.1$ | $0.0 \pm 0.0$ | $1.0 \pm 0.3$ | $0.1 \pm 0.1$ | $0.0 \pm 0.0$ | $0.1 \pm 0.1$ | $0.8 \pm 0.1$ | $0.5 \pm 0.3$ |
| MS1M-Arcface | $9.1 \pm 1.1$ | $6.3 \pm 0.8$ | $17.8 \pm 1.0$ | $15.3 \pm 1.7$ | $0.0 \pm 0.0$ | $0.0 \pm 0.0$ | $0.1 \pm 0.1$ | $0.2 \pm 0.3$ | $0.0 \pm 0.0$ | $0.1 \pm 0.1$ | $0.4 \pm 0.2$ | $0.5 \pm 0.4$ |

TABLE III
1:N IDENTIFICATION RESULTS FOR ID-I-SPLIT- PROTOCOLS WITH AND WITHOUT ALIGNMENT

| Algorithm | ID-I-Split-Ep1 | | | | ID-I-Split-Ep2 | | | | ID-I-Split-Ep3 | | | |
|---|---|---|---|---|---|---|---|---|---|---|---|---|
| | rank-1 | | rank-5 | | rank-1 | | rank-5 | | rank-1 | | rank-5 | |
| | Without | With | Without | With | Without | With | Without | With | Without | With | Without | With |
| ArcFace(r34-amf) | 31.9 | 37.87 | 41.06 | 47.39 | 6.64 | 5.01 | 13.97 | 11.92 | 5.83 | 5.78 | 12.6 | 12.97 |
| ArcFace(r50-am-lfw) | 31.24 | 34.69 | 40.97 | 46.17 | 8.35 | 4.32 | 13.97 | 9.84 | 7.09 | 6.88 | 11.81 | 14.69 |
| ArcFace(r100-ii) | 37.51 | 33.31 | 47.32 | 43.73 | 11.41 | 6.56 | 18.57 | 14.51 | 11.18 | 8.59 | 21.89 | 16.72 |
| SphereFace | 34.95 | 48.21 | 45.34 | 57.65 | 3.58 | 5.53 | 7.67 | 11.23 | 5.2 | 5.31 | 8.66 | 14.22 |
| lightCNN-29-V2 | 80.54 | 78.18 | 86.4 | 86.07 | 59.11 | 48.7 | 74.79 | 67.88 | 61.89 | 56.25 | 78.11 | 70.63 |
| lightCNN-29 | 76.17 | 68.49 | 83.1 | 77.2 | 44.8 | 29.88 | 61.67 | 47.5 | 46.14 | 33.44 | 65.2 | 51.72 |
| lightCNN-9 | 60.26 | 59.45 | 69.41 | 69.22 | 19.25 | 14.85 | 34.07 | 30.57 | 24.25 | 17.81 | 40.16 | 35.31 |
| Balanced-Softmax | 36.44 | 38.93 | 48.31 | 49.35 | 6.98 | 5.18 | 14.31 | 10.88 | 5.67 | 6.25 | 17.01 | 13.59 |
| CASIA-Arcface | 23 | 27.12 | 32.23 | 37.21 | 0.34 | 0.35 | 1.53 | 0.69 | 0.31 | 0.16 | 1.89 | 1.41 |
| CASIA-Softmax | 23.08 | 23.62 | 35.61 | 37.21 | 0.68 | 1.21 | 3.41 | 3.45 | 2.2 | 0.78 | 5.67 | 2.97 |
| Global-Softmax | 21.52 | 22.23 | 32.4 | 34.2 | 2.39 | 1.21 | 6.3 | 4.66 | 1.89 | 2.19 | 6.14 | 6.72 |
| MS1M-Arcface | 23.17 | 18.73 | 32.65 | 28.58 | 3.07 | 3.28 | 7.67 | 7.43 | 3.15 | 3.91 | 9.92 | 10.47 |

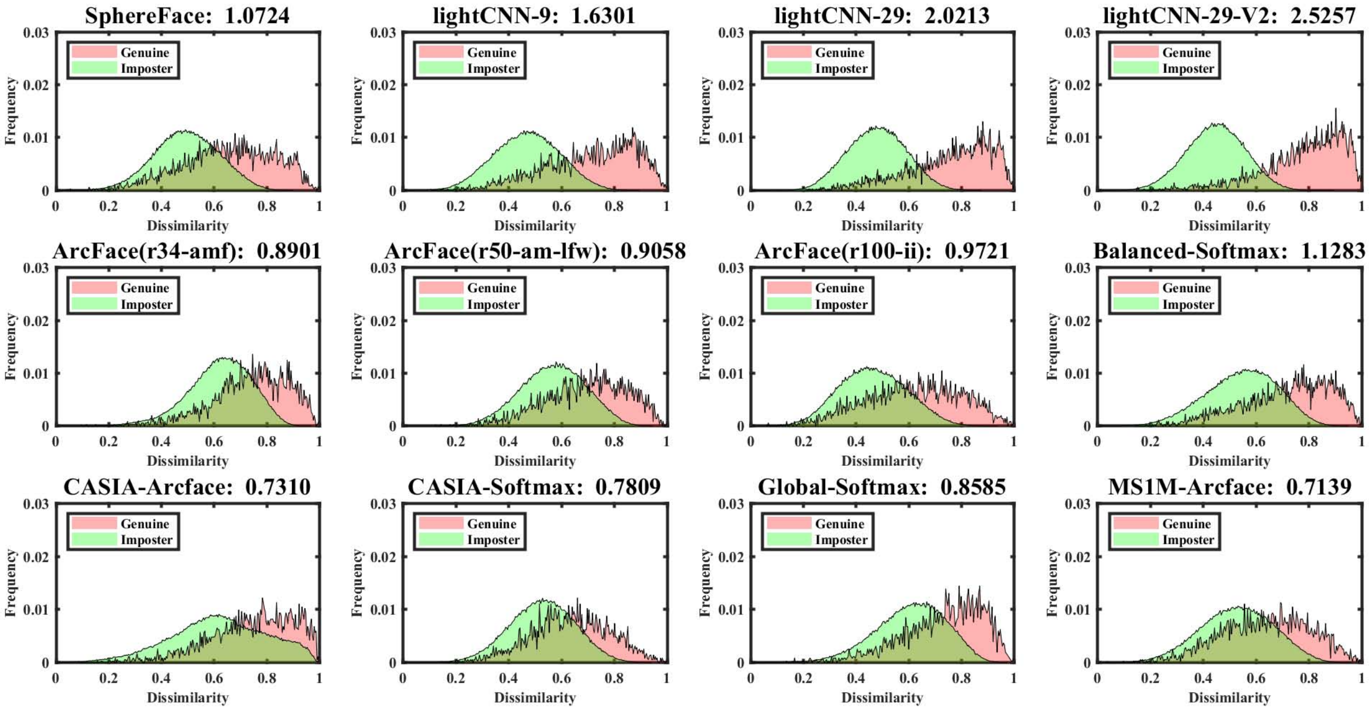


Fig. 2. DI values and genuine/impostor distributions of the baseline algorithms on aligned face images under ID-V-Split-Ep1

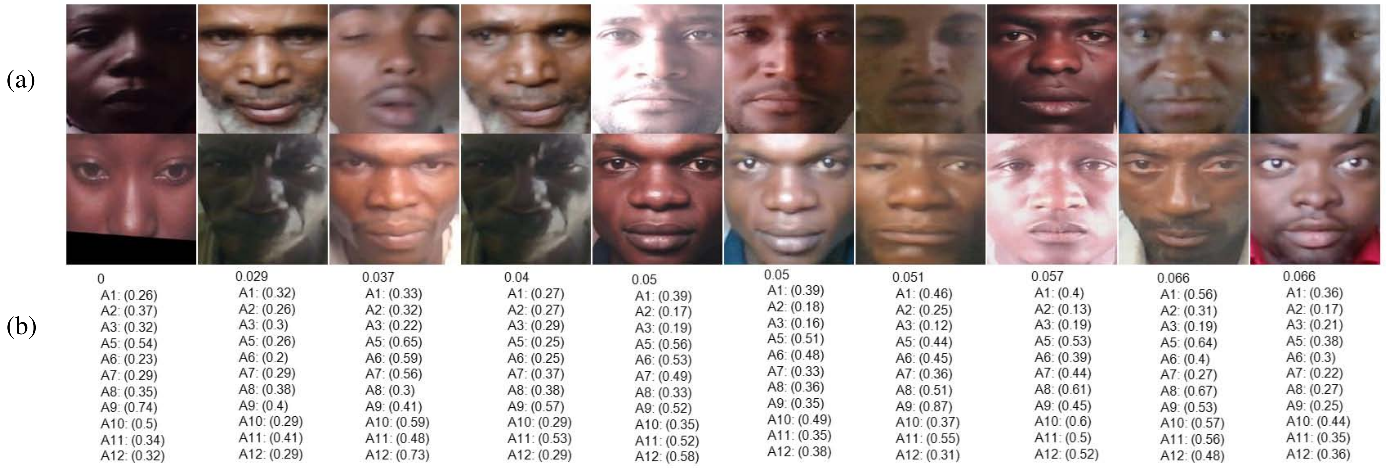


Fig. 3. Sample imposter pairs with similarity scores computed with *LightCNN-29-V2* (without A-tag) and other algorithms: A1-*SphereFace*, A2-*LightCNN-9*, A3-*LightCNN-29*, A5-*ArcFace-r34*, A6-*ArcFace-r50*, A7-*ArcFace-r100'*, A8-*Balanced-Softmax*, A9-*CASIA-Arcface*, A10-*CASIA-Softmax*, A11-*Global-Softmax*, A12-*MS1M-Arcface*

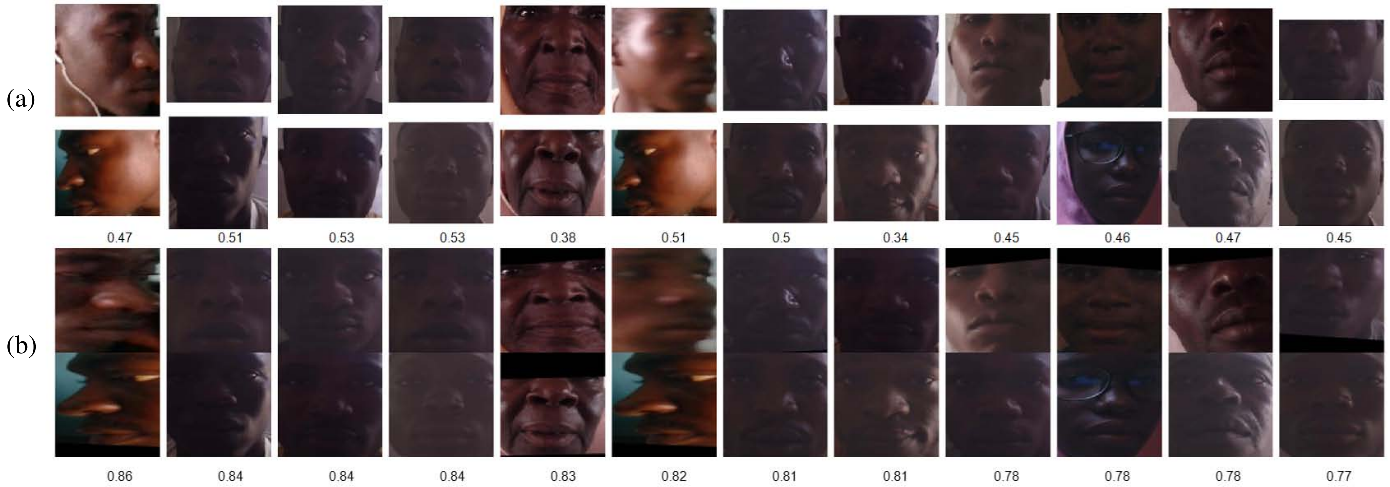


Fig. 4. Sample imposter pairs with their corresponding LightCNN similarity scores: (a) without alignment and (b) with alignment
